# Supplementary material for: Strain-induced structural change and nearly-commensurate diffuse scattering in the model high-temperature superconductor HgBa$_2$CuO$_{4+\delta}$
Source: arXiv:2510.21343 source file (2025-10-24)
Supplement: Supplementary file 1 [file SM.pdf]

# Supplemental Material for: Strain-induced structural change and nearly-commensurate diffuse scattering in the model high-temperature superconductor $HgBa_2CuO_{4+\delta}$

Mai Ye,[1,*] Wenshan Hong,[2,3] Tom Laurin Lacmann,[1,†] Mehdi Frachet,[1,‡] Igor Vinograd,[1,§] Gaston Garbarino,[4] Sofia-Michaela Souliou,[1] Michael Merz,[1,5] Rolf Heid,[1] Amir-Abbas Haghighirad,[1] Yuan Li,[2,3] and Matthieu Le Tacon[1,¶]

[1] Institute for Quantum Materials and Technologies, Karlsruhe Institute of Technology, Kaiserstr. 12, 76131 Karlsruhe, Germany
[2] International Center for Quantum Materials, School of Physics, Peking University, 100871 Beijing, China
[3] Beijing National Laboratory for Condensed Matter Physics, Institute of Physics, Chinese Academy of Sciences, Beijing 100190, China
[4] European Synchrotron Radiation Facility, BP 220, F-38043 Grenoble Cedex, France
[5] Karlsruhe Nano Micro Facility (KNMFi), Karlsruhe Institute of Technology, Kaiserstr. 12, 76131 Karlsruhe, Germany

## I. CRYSTALLOGRAPHIC DATA

The X-ray diffraction data used for structural analysis were taken at the European Synchrotron Radiation Facility (ESRF) ID15B beamline. The incident beam with photon energy of 30.0 keV was set to low flux and focused to a spot of 4 $\mu$m diameter. The diffracted beam was detected with a DECTRIS EIGER2 X 9M CdTe flat panel detector. Each diffraction image was recorded with an angular range of $\pm 35$ degrees and an angular step of 0.5 degrees. The measured XRD data are available from the ESRF Data Portal.

The software CrysAlisPro by Rigaku Oxford Diffraction was used for cell refinement and data reduction. The programs SHELXL and JANA were used to solve the crystal structure and perform relevant refinements. For each refinement, around 500 Bragg peaks were used. The data were corrected for Lorentz, polarization, extinction, and absorption effects. The automatic unit cell finding rendered a primitive tetragonal lattice when the strain was zero, and a primitive orthorhombic lattice when the sample was compressed. The data reduction results were inspected by the corresponding scale factor vs. frame plot. The strain values reported in this work are the real strain determined from the measured lattice parameters.

In Table. I and Table. II we present the crystallographic data of $HgBa_2CuO_{4+\delta}$ at 300 K (0% strain) and 78 K (0% strain and 1.1% strain) from the refinement of synchrotron x-ray diffraction data. The structures at zero strain have tetragonal symmetry, whereas the structure at 1.1% strain has a orthorhombic symmetry. The volume exhibits a small decrease under strain, consistent with the theory of elasticity because under approximations the relative change of the volume is proportional to $\epsilon_{aa}(1-\nu)$, where $\epsilon_{aa}$ is the strain in the $a$ direction (negative value) and $\nu$ is the effective Poisson ratio ($\nu_{ba}=0.16$ and $\nu_{ca}=0.11$, as given in the main text). The atomic displacement parameters (ADPs) shown in the table describe the thermal motion or static disorder of atoms around their mean positions. The ADPs were refined anisotropically, but due to space limitations only the equivalent values are listed in the table. The refinement also indicates around 4% vacancies at Hg sites, and around 0.09 oxygen doping level. To assess the quality and reliability of the refinements, the R1 factor ($R_1$) measures the discrepancy between observed and calculated structure factor amplitudes, the weighted R factor ($wR_2$) provides a similar but more statistically robust evaluation by applying intensity-based weighting, and the goodness of fit (GOF) quantifies how well the refined model explains the experimental data relative to the estimated uncertainties. The refinements fit well for all the three cases. The larger errors for the 1.1% strain case probably result from strain-induced disorder or inhomogeneity.

The Cu-O distances along the three directions measured at $T_c = 78$ K are listed in Table III. In both $a$ and $b$ directions, the Cu-O bond length and the lattice parameter have the same percentage changes. However, the out-of-plane Cu-O distance increases by 0.86% whereas the $c$-axis lattice parameter increases only by 0.12%. This difference indicates that under 1.1% strain, the $c$-axis Cu-O distance takes more portion from the $c$-axis lattice parameter than the $c$-axis Hg-O distance. The absolute change of the $c$-axis Cu-O distance, however, is only around 0.02 Å. Such a small absolute change may not lead to a significant change of the superconducting temperature.

* mai.ye@kit.edu
† Present address: Laboratory for Quantum Magnetism, Institute of Physics, École Polytechnique Fédérale de Lausanne, CH-1015 Lausanne, Switzerland
‡ Present address: Institut Néel CNRS/UGA UPR2940, 25 Rue des Martyrs, 38042 Grenoble, France
§ Present address: Laboratoire National des Champs Magnétigues Intenses, CNRS - Université Grenoble Alpes - Université Paul Sabatier - Institut National des Sciences Appliquées - European Magnetic Field Laboratory, 38042 Grenoble, France
¶ matthieu.letacon@kit.edu

TABLE I. Representative crystallographic data of $HgBa_2CuO_{4+\delta}$, determined from single-crystal synchrotron x-ray diffraction (part 1). The Wyckoff positions (Wyck.) are given for all atoms, and the occupancy (occ.) is given when a site is not fully occupied. The quantity $U_{\mathrm{equiv}}$ denotes the equivalent atomic displacement parameters. The errors shown are statistical errors from the refinement.

| Temp. (K) | | 300 K | 78 K | 78 K |
|---|---|---|---|---|
| Strain (%) | | 0 | 0 | 1.1 |
| Unit | Space group | $P4/mmm$ | $P4/mmm$ | $Pmmm$ |
| Cell | $a$ (Å) | 3.89000(10) | 3.88110(10) | 3.8384(3) |
| | $b$ (Å) | 3.89000(10) | 3.88110(10) | 3.889(3) |
| | $c$ (Å) | 9.5340(4) | 9.5096(4) | 9.5213(7) |
| | $\alpha$ (°) | 90 | 90 | 90 |
| | $\beta$ (°) | 90 | 90 | 90 |
| | $\gamma$ (°) | 90 | 90 | 90 |
| | V (Å$^3$) | 144.269(8) | 143.242(8) | 142.13(11) |
| Hg | Wyck. | 1$a$ | 1$a$ | 1$a$ |
| | $x$ | 0 | 0 | 0 |
| | $y$ | 0 | 0 | 0 |
| | $z$ | 0 | 0 | 0 |
| | occ. | | 0.96 | |
| | $U_{\mathrm{equiv}}$ (Å$^2$) | 0.01722(12) | 0.00837(14) | 0.0133(3) |
| Ba | Wyck. | 2$h$ | 2$h$ | 2$t$ |
| | $x$ | $\frac{1}{2}$ | $\frac{1}{2}$ | $\frac{1}{2}$ |
| | $y$ | $\frac{1}{2}$ | $\frac{1}{2}$ | $\frac{1}{2}$ |
| | $z$ | 0.29993(5) | 0.30001(6) | 0.29800(9) |
| | $U_{\mathrm{equiv}}$ (Å$^2$) | 0.01252(12) | 0.00745(15) | 0.0129(3) |
| Cu | Wyck. | 1$b$ | 1$b$ | 1$c$ |
| | $x$ | 0 | 0 | 0 |
| | $y$ | 0 | 0 | 0 |
| | $z$ | $\frac{1}{2}$ | $\frac{1}{2}$ | $\frac{1}{2}$ |
| | $U_{\mathrm{equiv}}$ (Å$^2$) | 0.0107(3) | 0.0067(3) | 0.0150(6) |
| O1 | Wyck. | 2$e$ | 2$e$ | 1$d$ |
| | $x$ | $\frac{1}{2}$ | $\frac{1}{2}$ | $\frac{1}{2}$ |
| | $y$ | 0 | 0 | 0 |
| | $z$ | $\frac{1}{2}$ | $\frac{1}{2}$ | $\frac{1}{2}$ |
| | $U_{\mathrm{equiv}}$ (Å$^2$) | 0.0109(13) | 0.0095(17) | 0.016(3) |
| O2 | Wyck. | 2$g$ | 2$g$ | 2$q$ |
| | $x$ | 0 | 0 | 0 |
| | $y$ | 0 | 0 | 0 |
| | $z$ | 0.2071(6) | 0.2066(8) | 0.2044(8) |
| | $U_{\mathrm{equiv}}$ (Å$^2$) | 0.0195(13) | 0.0118(15) | 0.0030(17) |
| O3 | Wyck. | 1$c$ | 1$c$ | 1$f$ |
| | $x$ | $\frac{1}{2}$ | $\frac{1}{2}$ | $\frac{1}{2}$ |
| | $y$ | $\frac{1}{2}$ | $\frac{1}{2}$ | $\frac{1}{2}$ |
| | $z$ | 0 | 0 | 0 |
| | occ. | | 0.09 | |
| | $U_{\mathrm{equiv}}$ (Å$^2$) | 0.01(14) | 0.008(12) | 0.0024 |
| O4 | Wyck. | N.A. | N.A. | 1$g$ |
| | $x$ | N.A. | N.A. | 0 |
| | $y$ | N.A. | N.A. | $\frac{1}{2}$ |
| | $z$ | N.A. | N.A. | $\frac{1}{2}$ |
| | $U_{\mathrm{equiv}}$ (Å$^2$) | N.A. | N.A. | 0.018(4) |

TABLE II. Representative crystallographic data of $HgBa_2CuO_{4+\delta}$, determined from single-crystal synchrotron x-ray diffraction (part 1). The Wyckoff positions (Wyck.) are given for all atoms, and the occupancy (occ.) is given when a site is not fully occupied. The quantity $U_{\mathrm{equiv}}$ denotes the equivalent atomic displacement parameters. The errors shown are statistical errors from the refinement.

| Temp. (K) | | 300 K | 78 K | 78 K |
|---|---|---|---|---|
| Strain (%) | | 0 | 0 | 1.1 |
| | GOF | 1.32 | 1.62 | 1.81 |
| | $wR_2$ (%) | 1.92 | 2.38 | 5.58 |
| | $R_1$ (%) | 1.69 | 2.07 | 2.47 |

TABLE III. The Cu-O distances at $T_c = 78$ K as a function of $a$-axis compressive strain along three directions. The unit for length is Å. The relative change with respect to zero-strain value is also indicated.

| Crystal Axis | 0.0% strain | 1.1% strain | Change |
|---|---|---|---|
| $a$ | 1.9405(1) | 1.9192(3) | -1.10% |
| $b$ | 1.9405(1) | 1.945(3) | +0.20% |
| $c$ | 2.790(8) | 2.814(8) | +0.86% |
